# Supplementary material for: Emergence of economic and social disparities through competitive gift-giving
Source: arXiv:2303.08424 source file (2024-07-02)
Supplement: Supplementary file 1 [file gift_phys_SI.pdf]

# Supplementary Information for: Emergence of Economic and Social Disparities by Gift Interactions

Kenji Itao and Kunihiko Kaneko

March 15, 2023

## Analytical estimation of social change

Here, we analyze how the distribution of the reputation score  $P(s)$  shifts between exponential and power law with the change in  $rl$ . Scores increase upon receipt of gifts, reciprocation, or repayment of debts. One acquires credit when the interest  $rw_i$  exceeds the recipient's wealth  $w_j$ . Debtors repay  $1/l$  of wealth while creditors acquire  $1/l$  of score in each step. Hence, creditors acquire  $|rw_i - w_j|_+ (= \max(0, rw_i - w_j))$  of score when the repayment is completed. However, because  $j$  may die before completing the repayment and  $j$ 's life expectancy is  $l$ , the expected increase in the score from the transaction is given by  $\min(|rw_i - w_j|_+, 1)$ . Therefore, the time development of the score is given by

$$\dot{s}_i = 1/l + \sum \eta/l + \min(|rw_i - w_j|_+, 1). \quad (1)$$

Recall that economic disparity, characterized by  $\alpha_w$ , evolves with  $rl$ , and that  $rl > 1$  provides a basic condition for the frequent incurrence of debts. Hence, as  $rl$  increases,  $|rw_i - w_j|_+$  increases, and the score distributions change.

When  $rl < 1$ , most gifts are reciprocated immediately. In other words,  $rw_i - w_j$  is generally negative and the third term in eq. (1) is negligible. Then,  $\langle s \rangle = 2/l$  and  $\dot{s}_i = 2/l$ . Accordingly,  $s_i = 2t/l$ , where  $t$  is  $i$ 's age. Since the age distribution is  $P(t) = \exp(-t/l)/l$ , the score distribution is  $P(s) = \exp(-s/2)/2$ .

When  $rl > 1$ , some gifts are not reciprocated. Hence,  $\min(|rw_i - w_j|_+, 1) = rw_i - w_j$  as long as the debt is repayable before death. Note that individuals acquire credit only if they give to those who have insufficient wealth. By denoting its probability as  $p$  and averaging the stochastic term, we obtain the following estimate:

$$\langle \dot{s}_i \rangle = 2/l + p|rw_i - \langle w \rangle|_+, \quad (2)$$

$$= 2/l + p|\dot{w}_i - 1 + r - 1/l|_+. \quad (3)$$

Hence,  $\dot{s} \rightarrow p\dot{w}$  if  $\dot{w} \gg 1$ . For  $rl > 1$ , since wealth distribution follows a power law, score distribution also follows a power law. However,  $\dot{s} \rightarrow 2/l$  for small  $\dot{w} (< 2/l)$ . Therefore, the score distribution has more middle classes than the wealth distribution, resulting in  $\alpha_s > \alpha_w$  (see Figs. 1 and 2). The transition of the score distribution from exponential to power law at  $rl \simeq 1$  is consistent with the simulation results in Fig. 2. Hence, the score distribution is exponential at  $rl \simeq 0.25$ , which validates the ignorance of connection bias in the analysis of economic change, down to such  $rl$  values.

When  $rl$  is sufficiently large, debtors often die before completing repayment. Hence, the expected increment of score from credit is generally  $\min(rw_i - w_j, 1) = 1$ , and thus  $\langle \dot{s}_i \rangle = 2/l + p$ , leading to

$$s_i = pt + 2t/l \simeq pt. \quad (4)$$

Hence, the score distribution reverts to exponential if the distribution of  $t$  is exponential. Here,  $t$  indicates the number of gifts that one makes, which is generally different from the age, in contrast to the case with  $rl < 1$ . If individuals receive gifts from the rich, they will need many time steps for repayment and will no longer earn scores. Note that once individuals are debtors, their social connections to the rich are strengthened by local preferential attachment. Since rich people can reciprocate gifts, they will no longer earn a score, even after finishing repayment. Hence,  $t$  generally equals the time that passes before an individual receives a gift from the richest individual. As the rich choose recipients randomly from  $N$  individuals, the distribution of  $t$  is determined by  $P(t) = \exp(-t/N)/N$ . Subsequently, the score distribution, except for the richest, is  $P(s) = \exp(-s/pN)/pN$ . On the other hand, the expected value

of  $t$  for the richest individual is the lifetime  $l$ . Hence, the score distribution will be exponential, with a half-life proportional to  $N$  for most individuals and  $l$  for the richest. Note that the gifts from the moderately rich may be repayable, and the score distribution for the middle class still follows the power law since  $\min(|rw_i - w_j|_+, 1) = rw_i - w_j$ . Additionally, the richest individual (monarch) cannot find debtors if all the others are already his/her debtors. Therefore, the largest score is bounded by  $\mathcal{O}(N)$ . Numerical results for different values of  $N$  (Fig. S2) show that  $\max \beta_s \simeq 0.2N$ , indicating that  $p \simeq 0.2$ .

## Supplementary figures

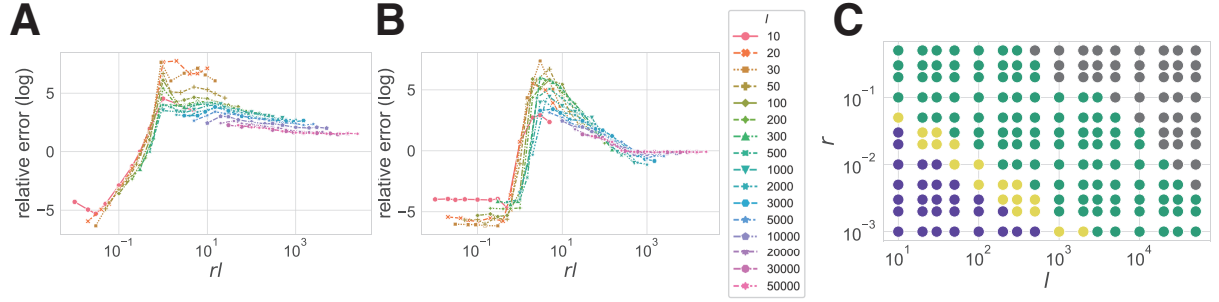

Figure S1: Statistical characteristics of the simulation results. (A) Relative error of power-law and exponential fitting for wealth  $RE_w$ . The logarithm of the relative error is obtained by fitting the top 30% with exponential and power-law distributions. The positive value indicates that power-law fitting is more appropriate than exponential fitting. (B) Relative error of power-law and exponential fitting for reputation score  $RE_s$ . (C) Phase diagram. The figure shows the parameter regions for  $RE_w, RE_s < 0$  (purple);  $RE_w \geq 0$  and  $RE_s < 0$  (yellow);  $RE_w, RE_s \geq 0$  (green);  $RE_w \geq 0$  and  $RE_s < 0$  with the monarch (grey), which gives almost the same diagram as in Fig. 2.

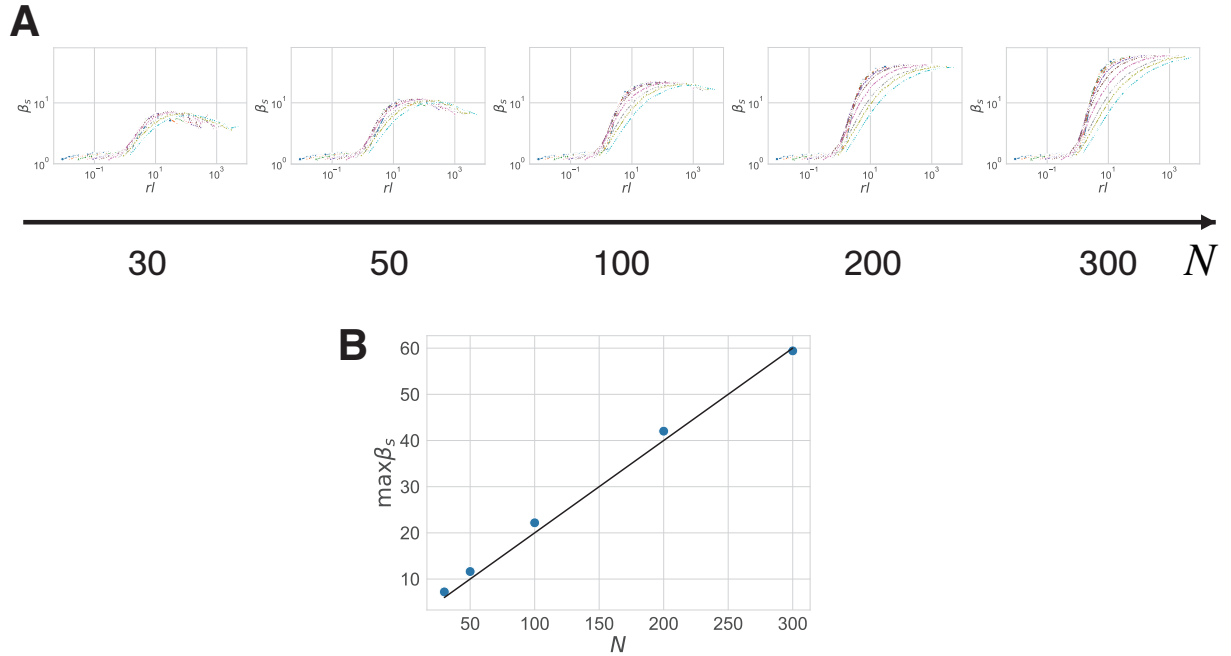

Figure S2: Dependence of half-life of score distribution  $\beta_s$  on population size  $N$ . (A) Dependence of  $\beta_s$  on  $rl$  for different population size  $N$ . (B) The relationship between  $\max \beta_s$  and  $N$ . The black solid line is the regression line  $\max \beta_s = 0.2N$ .
